# Supplementary material for: Active Crowd Counting with Limited Supervision
Source: arXiv:2007.06334 source file (2020-07-14)
Supplement: Supplementary file 1 [file sec-appendix.tex]

\appendix \label{Sec:Perspective}
%\holger{Headline should just be appendix and perspective estimation a section below that.}
%This appendix details the computation of $\frac{{\partial {L_{{\mathrm D}}}}}{{\partial {\alpha}}}$ and $\frac{{\partial {L_{{\mathrm D}}}}}{{\partial {\beta}}}$ ($t$ is omitted for simplicity) in (\ref{Eq:paraupdate}). Recalling the notations in (\ref{Eq:DensityWeight})(\ref{Eq:Weight}) and Sec.~\ref{Sec:Architecture}, we write out the chain rule:
%\begin{equation}\label{Eqn: diffalpha}
%\begin{aligned}
%\frac{{\partial {L}}}{{\partial \alpha }} &= \frac{{\partial L}}{{\partial {D^e}}}\frac{{\partial {D^e}}}{{\partial W}}\frac{{\partial W}}{{\partial \alpha }}\\
% &= \frac{{\partial L}}{{\partial {D^e}}}({D^{{e_1}}} - {D^{{e_2}}})\frac{{\partial W}}{{\partial \alpha }}\\
% &= \frac{{\partial L}}{{\partial {D^e}}}\sum\nolimits_j {(d_j^{{e_1}} - d_j^{{e_2}})} \frac{{\partial {w_j}}}{{\partial \alpha }}\\
% &= \frac{{\partial L}}{{\partial {D^e}}}\sum\nolimits_j {(d_j^{{e_1}} - d_j^{{e_2}})(p_j^e - \beta )f(p_j^e)(1 - f(p_j^e))}
%\end{aligned}
%\end{equation}
%Similarly, we have
%\begin{equation}\label{Eqn: diffbeta}
%\begin{aligned}
%\frac{{\partial {L}}}{{\partial \beta }} = \frac{{\partial L}}{{\partial {D^e}}} \sum\nolimits_j (d_j^{{e_1}} - d_j^{{e_2}})( - \alpha )f(p_j^e)(1 - f(p_j^e))
%\end{aligned}
%\end{equation}
This appendix provides the experimental results for perspective estimations.
%\section{Perspective estimations}
We evaluate perspective estimations on ShanghaiTech dataset~\cite{zhang2016cvpr}. We follow the same implementation details as in Sec.~\ref{Sec:ExperimentalDetails}. We first present the evaluation protocol and then offer the results.
\medskip 
 
\para{Evaluation Protocol.} The perspective maps produced by PACNN are of $\frac{1}{8}$ resolution of the ground truth maps. To compare with the ground truth, we downsample the ground truth maps to have the same resolution with the estimated maps. We normalize both the estimated and ground truth perspective values within each map for comparison.

\begin{table}[t]
	\setlength{\tabcolsep}{2.6pt}
	\centering
	\small
	\begin{tabular}{|c|c|c|c|}
		\hline
		ShanghaiTech &  $\overline {\mathrm{MAE_P}}$ & $\overline {\mathrm{RMSE_P}}$ & $\overline {\mathrm{PSNR_P}}$ \\
		\hline
		PartA& 0.092 & 0.120 & 18.06\\
		PartB & 0.116  &  0.149 & 16.83 \\
		\hline
	\end{tabular}
	%   \pretabspace
	\caption{Perspective estimations using PACNN. $\overline {\mathrm{MAE_P}}$, $\overline {\mathrm{RMSE_P}}$ and $\overline {\mathrm{PSNR_P}}$ are the average values of MAE$_\text P$, RMSE$_\text P$, and PSNR$_\text P$ over the dataset.}
	\label{Tab:Perspective}
	%   \posttabspace
\end{table}

%(${p_j} \leftarrow  \frac{{{p_j} - {{\min }_p}}}{{{{\max }_p} - {{\min }_p}}}$).

For each estimated perspective map $P^e$, we employ three measurements to evaluate its similarity to the ground truth $P^g$:
mean absolute perspective error (MAE$_\text P$), root mean square perspective error (RMSE$_\text P$), and peak perspective signal to noise ratio (PSNR$_\text P$),
\begin{equation}\label{Eq:MAE}
\begin{split}
&\mathrm{MAE_P} = \frac{1}{{S}}\sum\limits_{j = 1}^S {|{{p^e_j} - {p^g_j}}|},\\
&\mathrm{RMSE_P} = \sqrt{\frac{1}{{S}}\sum\limits_{j = 1}^S {({{p^e_j} - {p^g_j}})^2}},\\
&\mathrm{PSNR_P} = 20 \log_{10} (\frac{\mathrm{MAX_P}}{\mathrm{RMSE_P}})
\end{split}
\end{equation}
where $p^e_j$ and $p^g_j$ denote the normalized estimated and ground truth perspective values at pixel $j$, respectively. We use $S$ to denote the total number of pixels in each map. $\mathrm{MAX_P}$ is the maximum possible pixel value of the perspective map $P$. Since both $P^e$ and $P^g$ are normalized,  $\mathrm{MAX_P} = 1$ in practice. We average the MAE$_\text P$, RMSE$_\text P$ and PSNR$_\text P$ over the entire set, and denote by $\overline {\mathrm{MAE_P}}$, $\overline {\mathrm{RMSE_P}}$ and $\overline {\mathrm{PSNR_P}}$ our final measurements. Small $\overline {\mathrm{MAE_P}}$ and $\overline {\mathrm{RMSE_P}}$ and big $\overline {\mathrm{PSNR_P}}$ indicate good performance.
\medskip

\begin{table}[t]
	\setlength{\tabcolsep}{2.6pt}
	\centering
	\small
	\begin{tabular}{|c||c|c|c|}
		\hline
	 Examples in Fig.~\ref{Fig:PMAP} &  $ {\mathrm{MAE_P}}$ & ${\mathrm{RMSE_P}}$ & $ {\mathrm{PSNR_P}}$ \\
		\hline
		top-left& 0.093& 0.129 & 17.80\\
		top-right & 0.075 & 0.089 & 20.50 \\
		bottom-left& 0.090 & 0.121 & 18.31\\
		bottom-right & 0.126  & 0.152 & 16.40 \\
		\hline
	\end{tabular}
	%   \pretabspace
	\caption{Evaluations of Examples in Fig.~\ref{Fig:PMAP}. ${\mathrm{MAE_P}}$, ${\mathrm{RMSE_P}}$ and $ {\mathrm{PSNR_P}}$ are reported.}
	\label{Tab:Example}
	%   \posttabspace
\end{table}

\para{Results on ShanghaiTech.} We show the perspective map estimation results in Table~\ref{Tab:Perspective} on ShanghaiTech PartA and PartB, respectively. $\overline {\mathrm{MAE_P}}$, $\overline {\mathrm{RMSE_P}}$ and $\overline {\mathrm{PSNR_P}}$ are similar between PartA and PartB. Their $\overline {\mathrm{PSNR_P}}$ are 18.06, and 16.83, respectively. We illustrate some examples in Fig.~\ref{Fig:PMAP} and compute their MAE$_\text P$, RMSE$_\text P$ and PSNR$_\text P$, respectively in Table~\ref{Tab:Example}.
%; Top left: 0.093 (MAE$_\text P$), 0.129 (RMSE$_\text P$), 17.80 (PSNR$_\text P$); Top right: 0.075, 0.089, 20.5; Bottom left: 0.090, 0.121, 18.31; Bottom right: 0.126, 0.152, 16.4.  
The estimated perspective map in general keeps the color gradient as in the corresponding ground truth, albeit the noise. In Table.~\ref{Tab:Shanghaitech} we show the crowd counting accuracy using the estimated perspective maps is in fact very close to that using the ground truth perspective maps.
%\holger{Only use the word precision if you mean the same as in precision and recall.}
